# Supplementary material for: Search for $D^{*}(2007)^0\to\mu^+\mu^-$ in $B^-\to\pi^-\mu^+\mu^-$ decays
Source: arXiv:2304.01981 source file (2023-08-15)
Supplement: Supplementary file 1 [file appendix.tex]

% ===============================================================================
% Purpose: appendix to the standard template: standard symbol alises from Ulrik
% Author: Tomasz Skwarnicki
% Created on: 2009-09-24
% ===============================================================================

%{\noindent\normalfont\bfseries\Large Appendices}
\section*{Appendices}

\appendix
